# Supplementary material for: Security Properties for Open-Source Hardware Designs
Source: arXiv:2412.08769 source file (2024-12-16)
Supplement: Supplementary file 1 [file appendix.tex]

\onecolumn
\appendix

\section{Literature Review Included Papers}
\begin{table*}[h!]
  \centering
    \begin{tabular}{m{14cm}m{1.5cm}m{1.5cm}}
        \toprule
        Paper Title & Paper Type & Citation \\
\midrule
        HardFails: Insights into Software-Exploitable Hardware Bugs & \FV & ~\cite{dessouky2019fails} \\
        RTL-ConTest: Concolic Testing on RTL for Detecting Security Vulnerabilities & \FV & ~\cite{meng2021rtl} \\
        End-to-End Automated Exploit Generation for Validating the Security of Processor Designs & \FV & ~\cite{zhang2018end} \\
        Design of Access Control Mechanisms in Systems-on-Chip with Formal Integrity Guarantees & \FV & ~\cite{mehmedagic2023design} \\
        DIVAS: An LLM-based End-to-End Framework for SoC Security Analysis and Policy-based Protection & \PG & ~\cite{paria2023divas} \\
        A Formal Approach to Confidentiality Verification in SoCs at the Register Transfer Level & \FV & ~\cite{muller2021formal} \\
        Isadora: automated information-flow property generation for hardware security verification & \PG & ~\cite{deutschbein2021isadora} \\
        Transys: Leveraging Common Security Properties Across Hardware Designs & \PG & ~\cite{zhang2020transys} \\
        SPECS: A Lightweight Runtime Mechanism for Protecting Software from Security-Critical Processor Bugs & \FV & ~\cite{hicks2015specs} \\
        AGILE: Automated Assertion Generation to Detect Information Leakage Vulnerabilities & \FV + \PG & ~\cite{dipu2023agile} \\
        SoC Security Verification using Property Checking & \FV & ~\cite{9000170} \\
        Evaluating Security Specification Mining for a CISC Architecture & \PG & ~\cite{deutschbein2020evaluating} \\
        Fault Attacks on Access Control in Processors: Threat, Formal Analysis and Microarchitectural Mitigation & \FV & ~\cite{anton2023fault} \\
        LLM-assisted Generation of Hardware Assertions & \PG & ~\cite{kande2023llm} \\
        HUnTer: Hardware Underneath Trigger for Exploiting SoC-level Vulnerabilities & \FV & ~\cite{rajendran2023hunter} \\
        Sylvia: Countering the Path Explosion Problem in the Symbolic Execution of Hardware Designs & \FV & ~\cite{ryan2023sylvia} \\
        Countering the Path Explosion Problem in the Symbolic Execution of Hardware Designs & \FV & ~\cite{ryan2023countering} \\
        Applying Unique Program Execution Checking in the development flow of
        industrial IoT devices to prevent && \\  \quad vulnerabilities for side-channel attacks & \FV & ~\cite{solem2023applying} \\
        Mining Secure Behavior of Hardware Designs & \PG & ~\cite{deutschbein2021mining} \\
        Unique Program Execution Checking: A Novel Approach for Formal Security Analysis of Hardware & \FV & ~\cite{rahmani2022unique} \\
        Unlocking Hardware Security Assurance: The Potential of LLMs & \PG & ~\cite{meng2023unlocking} \\
        Exploring the Abyss? Unveiling Systems-on-Chip Hardware Vulnerabilities beneath Software & \FV & ~\cite{rajendran2024exploring} \\
        Ensuring Hardware Robustness via Security Verification & \FV & ~\cite{meng2023ensuring} \\
        WASIM: A Word-level Abstract Symbolic Simulation Framework for Hardware Formal Verification & \FV & ~\cite{fang2023wasim} \\
        Register transfer level information flow tracking for provably secure hardware design & \FV & ~\cite{7927266} \\
        Hardware verification using software analyzers & \FV & ~\cite{7308670} \\
        Property specific information flow analysis for hardware security verification & \FV & ~\cite{8587741} \\
        Automated test generation for activation of assertions in RTL models & \FV & ~\cite{shen2018symbolic} \\
\bottomrule
    \end{tabular}
    \caption{Papers included in our literature review. \FV indicates 
    papers that perform formal verification. \PG indicates papers that perform
    automated property generation.}
    \label{tab:papers}
\end{table*}
